# Supplementary material for: Quantitative Assessment of the Toner and Tu Theory of Polar Flocks
Source: arXiv:1908.03794 ancillary file (2019-08-10)
Supplement: Supplementary file 1 [file SUP_Toner_Tu_Arxiv_sub.pdf]

# Quantitative Assessment of the Toner and Tu Theory of Polar Flocks – Supplementary information –


Benoît Mahault,[1,2] Francesco Ginelli,[3] and Hugues Chaté[1,4,5]

[1] *Service de Physique de l'Etat Condensé, CEA, CNRS, Université Paris-Saclay, CEA-Saclay, 91191 Gif-sur-Yvette, France*
[2] *Max Planck Institute for Dynamics and Self-Organization (MPIDS), 37077 Göttingen, Germany*
[3] *Department of Physics and Institute for Complex Systems and Mathematical Biology, Kings College, University of Aberdeen, Aberdeen AB24 3UE, United Kingdom*
[4] *Beijing Computational Science Research Center, Beijing 100094, China*
[5] *LPTMC, CNRS UMR 7600, Université Pierre et Marie Curie, 75252 Paris, France*



(Dated: August 10, 2019)


## I. NUMERICAL METHODS

We first present details on how the density and velocity correlation functions were computed, and compare different schemes for the simulation of the Vicsek model. We mainly show results in 2D for concision, but similar conclusions were reached in 3D.

### A. Measurement of anisotropic correlations

Two-point density and velocity correlation functions were obtained by coarse-graining the corresponding fields on boxes of linear size 1. We checked that this choice does not influence our results, at least for the largest scales (not shown). From [1, 2], correlations are predicted to scale anisotropically w.r.t. the global polar order direction $\Phi$. One must thus 'keep track' of $\Phi$. To avoid measuring isotropic correlations, three strategies have been explored, which we detail now.

*Rotating the system.* In periodic boxes, $\Phi$ is free to rotate and its direction diffuses as shown in Fig. 1(a). One way to follow $\Phi$ is to rotate a copy of the system at each measure, so that the direction of the order is kept fixed. While this method does not affect the dynamics, it requires to average the data over considerably long times (the diffusion constant of $\Phi$ varies like $1/N$, with $N$ the number of particles, Fig. 1(a)). Averaging on times larger than the timescale of the rotation at size $L = 1000$ in 2D typically requires $\gtrsim 10^8$ timesteps.

*Applying an external field* can ensure that the direction of the global order is maintained along a given direction $\hat{\mathbf{e}}_\parallel$. This can be achieved by adding $h\hat{\mathbf{e}}_\parallel$ to the velocity alignment rule. For same system size, timescales for a proper averaging of the data are then reduced by around two orders of magnitude, such that larger systems become accessible. However, an applied external field is expected to damp fluctuations on scales $q^{-1} > h^{-1/z}$ [3], i.e. those of interest to in the Toner Tu theory. One therefore needs to decrease the value of $h$ when increasing system size and check the convergence of the results as $h \to 0$.

*Imposing reflective boundary conditions* on $d-1$ direction(s), while the last one remains periodic forces the flock into a channel. This method leads to averaging times similar as when applying an external field to the system. However, as active particles tend to stay close to solid borders [4], the channel configuration generates inhomogeneous density profiles along the transverse axis (see inset of Fig. 1(b)). We thus chose to evaluate the

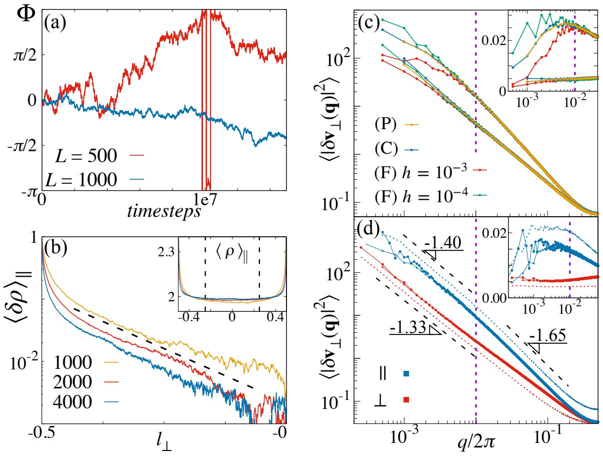


FIG. 1. (a): Direction of the global polar order $\Phi$ as function of time for simulations done with periodic boundary conditions. (b): Excess density at the solid boundaries averaged over the direction longitudinal to the order and time as function of the reduced length $l_\perp = |\mathbf{r}_\perp|/L - \frac{1}{2}$ in the channel configuration. The black dashed line indicates the exponential behavior with a characteristic length $\simeq 0.1 \times L$. Inset: full density profile, the vertical dashed lines mark the region where the fields are computed. (c): Equal-time velocity correlation functions computed in a periodic box rotating the system (P), applying an external field $h$ (F), and in a channel configuration (C). The upper and lower sets of curves respectively represent the functions in the longitudinal and transverse directions, for (P) $L = 1000$ and for (F) and (C) $L = 2000$. The curves have been shifted vertically to ensure the collapse. (d): Same as (c) but obtained from simulations of the Vicsek model with scalar (triangles: $L = 4000$, dots: $L = 8000$) and vectorial (dashed lines, $L = 8000$) noises in the channel geometry. In (c,d) the insets show the same curves rescaled by $\left(\frac{q}{2\pi}\right)^\sigma$ with $\sigma = 1.40$(longitudinal) and 1.33(transverse), and the vertical dashed purple lines mark the crossover scale $q_c/2\pi$ identified for vectorial noise (see text).

fields from one half of the total system only, excluding regions near the reflective walls. Computing the excess density $\delta\rho = \rho - \bar{\rho}$, where $\bar{\rho}$ denotes the field averaged over this central region, Fig. 1(b) shows that it exponentially decays with characteristic length $\simeq 0.1 \times L$ (this is also true in 3D, not shown), where $L$ denotes the linear system size. Perturbations introduced by the solid boundaries are thus local. We checked that varying reasonably the size of the region where the fields are computed does not affect our results (not shown).

Because of the walls, the fields are no more periodic in the transverse direction. We thus always considered arrays of transversal extension twice as large as necessary to fit in the data, and zero-padded the unused bins in order to avoid the occurrence of spurious correlations. This procedure was also applied in the "time direction" to the measure of space-time correlation functions.

We note that although the density in the bulk is mostly uniform, its value varies with system size (see insets of Fig. 1(b)). This explains why in 2D density correlations are more subjected to finite size effects in the transverse direction (see Fig. 1(c) of the main text).

Velocity and density equal-time correlation functions were evaluated using the three above-presented methods for linear system sizes 1000 and 2000. Fig. 1(c) shows that the corresponding curves mostly differ from each other by only a constant pre-factor, except when the applied external field $h$ is too strong which results as expected in a damping of correlations on the larger length-scales. In particular and despite the relatively small size considered, the crossover leading to a weakly anisotropic behavior of the velocity correlation function (see main text) is present regardless of the protocol employed for their measurement. We thus conclude that the three of them lead to similar results.

### B. Vicsek model with scalar noise

In the main text we present results obtained from simulations of the Vicsek model implemented with vectorial noise that it has been proven to be less sensitive to finite size effects [5] than its angular noise version, defined by

$$\hat{\mathbf{e}}_i^{t+1} = \mathcal{R}_\eta \circ \vartheta\left[\langle \hat{\mathbf{e}}_j^t \rangle_{j\sim i}\right] , \quad \mathbf{r}_i^{t+1} = \mathbf{r}_i^t + v_0 \hat{\mathbf{e}}_i^{t+1} , \qquad (1)$$

where $\vartheta[\mathbf{u}] = \mathbf{u}/|\mathbf{u}|$, $\langle . \rangle_{j\sim i}$ is the average over all particles $j$ within unit distance of $i$ (including $i$), and the operator $\mathcal{R}_\eta$ randomly rotates vectors uniformly in the interval $(-\pi\eta; \pi\eta]$ in 2D (the cap of surface $2\pi(1 - \cos(\eta))$ in 3D). We chose the parameters of the model such that the global order parameter $\Pi = |\langle \hat{\mathbf{e}}_i \rangle_i|$ takes similar steady-state values with the two rules ($\simeq 0.87$). For all runs with scalar noise, we chose $\rho_0 = 2$, $\eta = 0.2$ and $v_0 = 0.5$.

Fig. 1(d) compares the equal-time velocity correlation functions obtained from the scalar and vectorial noise schemes using the third method with solid boundaries. In the transverse direction (lower set of curves), the "scalar-noise" velocity correlation function does not scale as well as for vectorial noise. However, the last points we have indicate that it could reach a power law behavior for even larger systems with an exponent $-\zeta \simeq -1.33$ (see inset), in agreement with our results obtained with vectorial noise. In the longitudinal direction (upper set of curves), the function also experiences a crossover at $q_c^{\rm scal}$ smaller but of the order of that found with vectorial noise $q_c^{\rm vect} \simeq 10^{-2}$. At larger wavenumbers, it behaves as a power law with an exponent close to $-1.65$, although slightly smaller, and below the crossover it scales with an exponent compatible with $-1.40$. In both directions the small $q$ behavior of the velocity correlation function evaluated with scalar and vectorial noises are thus rather similar, although finite size effects seem to be more predominant for the former. Similar results are found from the density correlations and in 3D (not shown).

| | $d=2$ | | | $d=3$ | | |
|---|---|---|---|---|---|---|
| | TT95 | pre-c | post-c | TT95 | pre-c | post-c |
| $\chi$ | $-0.20$ | $\simeq -0.25$ | $-0.31(2)$ | $-0.60$ | $\simeq -0.57$ | $\simeq -0.62$ |
| $\xi$ | 0.60 | $\simeq 0.80$ | 0.95(2) | 0.80 | $\simeq 0.90$ | $\simeq 1$ |
| $\zeta$ | 1.20 | 1.33(2) | 1.33(2) | 1.60 | 1.77(3) | 1.77(3) |
| $z$ | 1.20 | 1.33(2) | 1.33(2) | 1.60 | $\simeq 1.77$ | $\simeq 1.77$ |
| $\alpha$ | 1.60 | 1.67(2) | 1.67(2) | 1.53 | 1.59(3) | 1.59(3) |
| $\nu$ | 1.33 | 1.38(2) | 1.33(2) | 1 | 1 | 1 |

TABLE I. Exponent values conjectured by Toner and Tu in [1] and those resulting from our numerical evaluation of the density and velocity correlation functions in the pre- and post-crossover regimes. $\zeta = d-1+2\chi+\xi$, $\alpha$ and $\nu$ respectively correspond to GNF and transverse super-diffusion and are defined in the text.

## II. GIANT NUMBER FLUCTUATIONS AND TRANSVERSE SUPERDIFFUSION

Giant number fluctuations in 2&3D, and superdiffusion in the direction transverse to the order in 2D are two important consequences of the TT theory [2, 6].

*GNF* The density correlation function averaged over all directions of $\mathbf{q}$ is predicted to scale as $q^{-\zeta}$ for at small $q$. Averaging our data over $\theta_{\mathbf{q}}$, we indeed find such a behavior with values of $\zeta$ compatible with the ones presented in the main text (not shown). Diverging density correlations for $q \to 0$ imply the presence of giant number fluctuations (GNF), i.e. that the variance of the number of particles $\langle \Delta n^2 \rangle$ evaluated in sub-domains containing on average $\langle n \rangle$ of them scales faster than $\langle n \rangle$. In this case, Toner and Tu theory predicts $\langle \Delta n^2 \rangle \sim \langle n \rangle^\alpha$ with $\alpha = 1 + \zeta/d$. Since our numerical estimations of $\zeta$ in 2&3D remain rather close to those they conjectured, the GNF exponents differ very little from their initially predicted values (see Table I). The computation of GNF in general only leads to limited accuracy in the determination of the corresponding exponent [7–9], such that they can't be used to discriminate between the two sets of numbers. In 2D, most of numerical studies found $\alpha \gtrsim 1.6$,

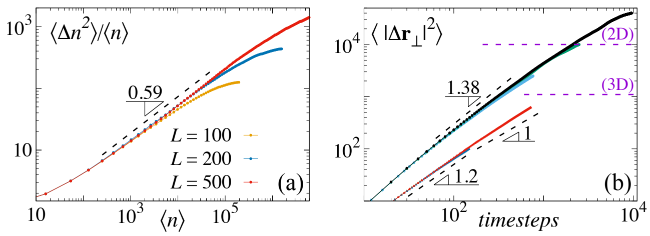


FIG. 2. (a): $\langle \Delta n^2 \rangle$ rescaled by $\langle n \rangle$ in 3D showing giant number fluctuations. (b): Transverse mean square displacement of particles in 2D (turquoise ($L = 1000$), green ($L = 2000$), and black ($L = 4000$) curves) and 3D (lower set of curves, same caption as (a)). The horizontal dashed purple lines mark the estimated crossover scales for both dimensions. All data correspond to vectorial noise with parameters $\rho_0 = 2$, $v_0 = 1$, $\eta = 0.5$(2D) and 0.45(3D).

which is compatible with our estimation $\alpha = 1.67(2)$. We also measured directly the GNF in 3D, Fig. 2(a) shows that the corresponding data is compatible with the value computed from the correlation functions: $\alpha = 1.59(3)$.

*Transverse superdiffusion* The scaling of velocity correlations imply that the mean-square displacement of particles computed in the direction(s) transverse to the global order $\langle |\Delta \mathbf{r}_\perp|^2 \rangle$ scales with time as $t^\nu$ with $\nu = 2(1 + \chi/\xi)$ if $2\chi/\xi > -1$, and 1 otherwise. The values of $\chi$ and $\xi$ conjectured by Toner and Tu then imply the that the motion of particles in the transverse direction(s) is superdiffusive in 2D, with an exponent $\nu = \frac{4}{3}$, and diffusive in 3D. Using the values determined from the equal-time correlation functions, we remarkably find, to numerical accuracy, values close, if not identical (see Table I).

We evaluated the transverse MSD of particles $\langle |\Delta \mathbf{r}_\perp|^2 \rangle$ from individual trajectories starting near the center of the channel at $t = 0$ in both 2&3D (see Fig. 2(b)). Even considering our largest sizes in 2D, we couldn't reach scales larger than the crossover to weak anisotropy in the velocity correlation scaling. Since $\nu$ explicitly depend on the anisotropy, we cannot expect to see its asymptotic value ($\simeq 1.33$), but rather the one corresponding to the values taken by $\chi$ and $\xi$ below the crossover ($\simeq 1.38$) The pre- and post-crossover estimates of $\nu$ are close from each other, and the data shown in Fig. 2(b) is compatible with $\nu \simeq 1.3 - 1.4$, but the scaling is not clean enough to distinguish between the two.

In 3D, our values of $\chi$ and $\xi$ below and above the crossover both imply $\nu = 1$. A direct measurement of $\langle |\Delta \mathbf{r}_\perp|^2 \rangle$ shows a power law behavior with an exponent $\nu \simeq 1.2$ that decreases at larger times. It is thus not excluded that normal diffusion is reached on scales larger than those currently accessible. In [8], a superdiffusive behavior of $\langle |\Delta \mathbf{r}_\perp|^2 \rangle$ with $\nu \simeq 1.7$ was reported for 3D flocks with cohesive interactions. This result, incompatible with the data of Fig. 2(b), could be due to the effect cohesion or to the fact that if not evaluated in a controlled geometry, $\langle |\Delta \mathbf{r}_\perp|^2 \rangle$ can easily get a ballistic component leading to spurious superdiffusion.

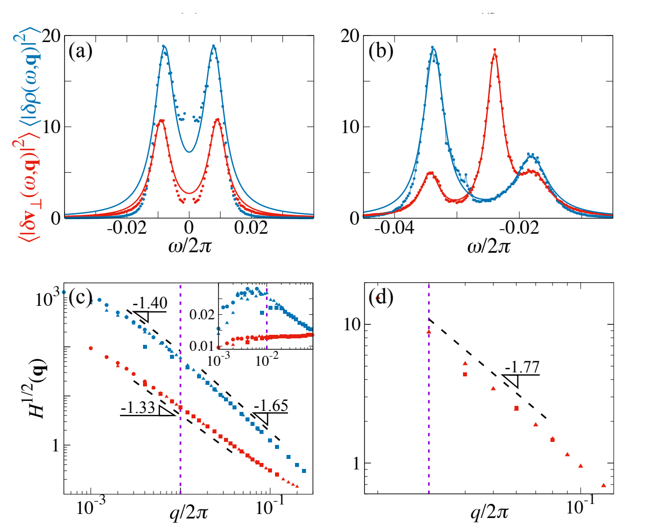


FIG. 3. (a,b): Density (blue) and velocity (red) space-time correlations as function of frequency $\omega$ in 2D for $\theta_\mathbf{q} = \frac{\pi}{2}$(a) and 3D for $\theta_\mathbf{q} = \frac{\pi}{4}$(b). For (a,b) $\frac{q}{2\pi} = 0.02$ and 0.03. The density curves have been rescaled vertically for clarity, and solid lines are fits by sums of Cauchy distributions (see text). (c,d): Scaling of the peaks heights with $q$ in the longitudinal (blue) and transverse (red) directions in 2D(c) and 3D(d). Inset of (c): Same curves but rescaled by $\left(\frac{q}{2\pi}\right)^\sigma$ with $\sigma = 1.40$ (longitudinal) and 1.33 (transverse). Squares, triangles and dots respectively correspond to $L = 1000$, 2000, 4000 (2D) and $L = 100$, 200 and 500 (3D). The vertical dashed purple lines mark the estimated crossover scales $q_c/(2\pi)$.

## III. SCALING OF VELOCITY PEAKS HEIGHTS

The peaks present in the density and velocity space-time correlation functions are in general well fitted by sums of Cauchy distributions of the type $H_{\pm,\mathrm{T}}(\mathbf{q}) \left[1 + (\omega - \omega^*_{\pm,\mathrm{T}}(\mathbf{q}))^2/\Delta\omega^2_{\pm,\mathrm{T}}(\mathbf{q})\right]^{-1}$ where $H_{\pm,\mathrm{T}}(\mathbf{q})$, $\omega^*_{\pm,\mathrm{T}}(\mathbf{q})$, and $\Delta\omega_{\pm,\mathrm{T}}(\mathbf{q})$ are all anisotropic functions that account for their heights, positions, and widths (see Figs. 3(a,b)). In the main text we present the scaling of the widths $\Delta\omega_{\pm,\mathrm{T}}(\mathbf{q})$, giving an estimation of the dynamical exponent $z$. $z$ can also be obtained from the heights $H_{\pm,\mathrm{T}}(\mathbf{q})$ of the peaks, which should scale as $q_\parallel^{-(z+\zeta)/\xi}$ and $q_\perp^{-(z+\zeta)}$ with $\zeta = d - 1 + 2\chi + \xi$ respectively in the longitudinal and transverse directions.

Moreover, our results related to $\Delta\omega_{\pm,\mathrm{T}}(\mathbf{q})$ give strong evidence that $z = \zeta$ in 2 and 3 dimensions. Fig. 3(c) shows that in 2D $H^{1/2}_{\pm,\mathrm{T}}(\mathbf{q})$ indeed scales with exponents similar to those of the equal-time velocity correlation function, with a quality comparable to the peak widths scaling (see Figs. 1(a) and 2(a) in the main text). In the transverse direction, we also find that $z = \zeta \simeq 1.33$, and partial evidence for a crossover scale $\ell_c \simeq 100$ such that $z/\xi \simeq 1.65$ for $q_\parallel > \ell_c^{-1}$ and $z/\xi \simeq 1.40$ for $q_\parallel < \ell_c^{-1}$. As for the other quantities we measured, results in 3D are more limited by finite size effects. We could nevertheless extract scalings laws for $H_{\pm,\mathrm{T}}(\mathbf{q})$ and $\Delta\omega_{\pm,\mathrm{T}}(\mathbf{q})$

(see main text for the latter) from the peak corresponding to the transverse component $\mathbf{v}_\mathrm{T}$ of $\delta\mathbf{v}_\perp$ for $\theta_\mathbf{q} = \frac{\pi}{2}$. Fig. 3(d) shows that $H^{1/2}_{\pm,\mathrm{T}}(\mathbf{q})$ scales with an exponent roughly compatible with 1.77, in agreement with our other results.

## IV. COMMENTS ON HYPERSCALING RELATIONS

In [10], seven relevant nonlinearities were found

$$\nabla_\perp \cdot (\delta\rho\delta\mathbf{v}_\perp)\,,\ \lambda_1 (\delta\mathbf{v}_\perp \cdot \nabla_\perp)\,\delta\mathbf{v}_\perp,\ g_3\nabla_\perp\delta\rho^2, \\ w_2\partial_\parallel\delta\rho^2,\ w_3\partial_\parallel \left|\delta\mathbf{v}_\perp\right|^2,\ g_1\delta\rho\partial_\parallel\delta\mathbf{v}_\perp,\ g_2\delta\mathbf{v}_\perp\partial_\parallel\delta\rho, \quad (2)$$

where $\partial_\parallel \equiv \nabla\cdot\hat{\mathbf{e}}_\parallel$, $\nabla_\perp \equiv \nabla - \partial_\parallel\hat{\mathbf{e}}_\parallel$, and all pre-factors are unimportant for the following and their definition can be found in [10]. In their initial papers [1, 2], Toner and Tu only considered the first three of these nonlinearities, which in 2D are all total $\perp$ derivatives (in 2D $\nabla_\perp = \partial_\perp\hat{\mathbf{e}}_\perp$ and the $\lambda_1$ term is $\lambda_1\partial_\perp\left|\delta\mathbf{v}_\perp\right|^2/2$). As a consequence, only terms themselves involving $\perp$ derivatives could be renormalized. Therefore, a few coefficients like the noise variance $\Sigma$ or the one associated with the longitudinal diffusion $D_\parallel\partial_\parallel^2\delta\mathbf{v}_\perp$ did not admit any graphical correction. Simple power counting for these two implies that

$$\frac{d\Sigma}{d\ell} = (z-\zeta+\mathrm{G}_\Sigma)\Sigma\,,\quad \frac{dD_\parallel}{d\ell} = (z-2\xi+\mathrm{G}_\parallel)D_\parallel\,, \quad (3)$$

where the "G" terms account for graphical corrections. Setting them to 0 and requiring that these coefficients flow to a fixed point leads to $z = \zeta = d-1+2\chi+\xi$ and $z = 2\xi$. Our numerical simulations give strong evidence that the first relation is satisfied while the second is not (see Table I).

$z=\zeta$ thus suggests that all relevant nonlinearities at the TT fixed point can be written as total $\parallel$ or $\perp$ derivatives. This way, the above argument still applies to $\Sigma$, which involves no derivatives, but not to the diffusion coefficient $D_\parallel$. On the contrary, if there were at least a relevant nonlinearity that could not be written as a total spatial derivative, it would renormalize the noise and $z=\zeta$ would not hold. Going back to Eq. (2), this reasoning means that the the $g_1$ and $g_2$ nonlinearities are likely to be irrelevant at the TT point (or that $g_1 = g_2$, which is not true at the linear fixed point).

When derived from microscopic models, hydrodynamic equations for active matter generally exhibit noise terms multiplicative in the density and order fields [11, 12], in contrast with the additive noise considered by Toner and Tu. Such terms in the velocity equation scaling like $|\mathbf{v}|^p \times \rho^q$ would be renormalized as in Eq. (3) but with a corresponding eigenvalue $z-\zeta+2\chi(p+q)$. If $z=\zeta$, nonlinearities do not renormalize multiplicative noise because of the same argument detailed above. Therefore, in 2D the multiplicative noise is marginal (at the linear fixed point $\chi_\mathrm{lin}=0$) and is irrelevant in 3D ($\chi_\mathrm{lin} = -\frac{1}{2}$). Moreover, our data in 2D and 3D do not show any qualitative difference, which seems to indicate that multiplicative noise can also be neglected in 2D.

The third hyperscaling relation derived by Toner and Tu ($z = 1-\chi$) came from the fact that in the first papers the hydrodynamic equations were invariant under the "Pseudo-Galilean" transformation: $\delta\mathbf{v}_\perp \to \delta\mathbf{v}_\perp + \mathbf{v}_\mathrm{PG}$ and $\mathbf{r} \to \mathbf{r} - \lambda_1\mathbf{v}_\mathrm{PG}t$, where $\mathbf{v}_\mathrm{PG}$ is a constant velocity in the transverse plane. Although the equations obtained after the reanalysis of [10] do not show this symmetry, we find to numerical accuracy that this hyperscaling relation is asymptotically satisfied in 2D while it is not in 3D (see the post-crossover values in Table I). At present, we do not have a theoretical argument justifying this result.


[1] J. Toner and Y. Tu, Long-Range Order in a Two-Dimensional Dynamical XY Model: How Birds Fly Together, Phys. Rev. Lett. **75**, 4326 (1995).

[2] J. Toner and Y. Tu, Flocks, herds, and schools: A quantitative theory of flocking, Phys. Rev. E **58**, 4828 (1998).

[3] N. Kyriakopoulos, F. Ginelli, and J. Toner, Leading birds by their beaks: the response of flocks to external perturbations, New Journal of Physics **18**, 073039 (2016).

[4] H. H. Wensink and H. Löwen, Aggregation of self-propelled colloidal rods near confining walls, Phys. Rev. E **78**, 031409 (2008).

[5] G. Grégoire and H. Chaté, Onset of collective and cohesive motion, Phys. Rev. Lett. **92**, 025702 (2004).

[6] F. Ginelli, The Physics of the Vicsek model, The European Physical Journal Special Topics **225**, 2099 (2016).

[7] H. Chaté, F. Ginelli, G. Grégoire, and F. Raynaud, Collective motion of self-propelled particles interacting without cohesion, Phys. Rev. E **77**, 046113 (2008).

[8] H. Chaté, F. Ginelli, G. Grégoire, F. Peruani, and F. Raynaud, Modeling collective motion: variations on the Vicsek model, The European Physical Journal B **64**, 451 (2008).

[9] S. Ngo, *Physique Statistique des Groupes en Mouvement*, Ph.D. thesis, Université Pierre et Marie Curie (2013).

[10] J. Toner, Reanalysis of the hydrodynamic theory of fluid, polar-ordered flocks, Phys. Rev. E **86**, 031918 (2012).

[11] F. D. C. Farrell, M. C. Marchetti, D. Marenduzzo, and J. Tailleur, Pattern Formation in Self-Propelled Particles with Density-Dependent Motility, Phys. Rev. Lett. **108**, 248101 (2012).

[12] E. Bertin, H. Chaté, F. Ginelli, S. Mishra, A. Peshkov, and S. Ramaswamy, Mesoscopic theory for fluctuating active nematics, New Journal of Physics **15**, 085032 (2013).
